# Supplementary material for: Glitch in Time: Exploiting Temporal Misalignment of IMU For Eavesdropping
Source: arXiv:2409.16438 source file (2025-01-13)
Supplement: Supplementary file 1 [file appendix.tex]

% \section{Overflow form other sections}
% \label{sec:set-diff-dodis}
% Sometime you ware super excited about some details that does not quite fit with
% the rest of the paper goes here. For example, some details about how you
% instrumented the Android Linux kernel should go to appendix, and for really
% curious reader to read. Remember it's appendix, so the reader is not required to
% read, and you should not put critical information in appendix that is crucial
% for understanding the rest of the paper.

%%% Local Variables:
%%% mode: latex
%%% TeX-master: "main"
%%% End:
